# Supplementary material for: Braids of Three Strands and Geodesics Shooting in $SL_2(\mathbb{R})$
Source: arXiv:2608.21484 source file (2026-08-21)
Supplement: Supplementary file 1 [file exeSols.tex]

\pagebreak

\section{INTERNAL: Exercises and Solutions}

FROM Sec.~\ref{sasMetricVer:sec}

\bigskip
{\sl Exercise:} Show that $\eta_{\SD}$ is the pullback of  $\eta_{\SH}$ via the map $\SD \to \SH$ induced by the M\"obius transformation $f_{\D,\H}: \D \to \H$. (Use the formulas from Sect.~\ref{DHpassage:sec}.) 
\medskip

{\sl Solution to Exercise:}
We dutifully transform the pieces of $\eta_{\SH}$ and assemble at the end.  
First, invoking (\ref{dotthetaphi:eq}) (in Leibniz notation), we record
\begin{align}\label{dthe:eq}
  d\theta 
  = 2 \Im\left(\frac{1}{1-w}  dw \right)  + d\phi.
  \end{align}
 Likewise, (\ref{zwthetaphi:eq}) gives 
  \begin{align} \Re(dz) = \Re\left( \frac{2\iota}{(1 - w)^2} dw \right)
    = - 2 \Im\left( \frac{(1-\overline{w})^2}{|1 - w|^4} dw \right).
  \end{align}
Combine this with 
  \begin{align}
    \Im(z) = \Im\left( \iota \frac{1+w}{1-w} \right) = \Re\left( \frac{(1+w)(1-\overline{w})}{|1-w|^2} \right)
    = \frac{1-|w|^2}{|1-w|^2}
  \end{align}
  to obtain 
  \begin{align}
    \label{rdzim:eq}
    \frac{\Re(dz)}{\Im(z)}
    = -2 \Im\left( \frac{(1-\overline{w})^2 dw}{(1-|w|^2)|1-w|^2} \right)
    = -2 \Im\left( \frac{1-\overline{w}}{(1-w) (1-|w|^2)}  dw \right).
  \end{align}
 Finally, the transformed $\eta_{\SH}$ comes from adding (\ref{dthe:eq}) and (\ref{rdzim:eq}) and one sees that the right sides combine to  match $\eta_{\SD}$ due to the identity  (cf.\ Lemma~\ref{magicMobIdent:lem})
  \begin{align}
    \frac{1}{1-w} - \frac{1-\overline{w}}{(1-w)(1-|w|^2)}
    = \frac{1-|w|^2 - 1 + \overline{w}}{(1-w)(1-|w|^2)} = \frac{\overline{w}(1-w)}{(1-w)(1-|w|^2)}
    = \frac{\overline{w}}{1-|w|^2}.
  \end{align}
$\Box$
\medskip

%%% Local Variables: 
%%% mode: latex
%%% TeX-master: "../mShort.tex"
%%% End: 
